# Supplementary material for: MVDiffusion++: A Dense High-resolution Multi-view Diffusion Model for Single or Sparse-view 3D Object Reconstruction
Source: arXiv:2402.12712 source file (2024-04-30)
Supplement: Supplementary file 2 [file single_view_reconstruction.tex]

\section{Addition results on single view reconstruction}

\begin{figure}
    \centering
    \includegraphics[width=\textwidth]{assets/gso_0.pdf}
    \includegraphics[width=\textwidth]{assets/gso_1.pdf}
    \caption{Caption}
    \label{fig:enter-label}
\end{figure}
