# Supplementary material for: MVDiffusion++: A Dense High-resolution Multi-view Diffusion Model for Single or Sparse-view 3D Object Reconstruction
Source: arXiv:2402.12712 source file (2024-04-30)
Supplement: Supplementary file 3 [file view_dropout_analysis.tex]

\section{View dropout analysis}

\section{implementation details}
%\mypara{Mask-aware VAE fine-tuning }
%We finetune the M-VAE with around 3 million RGBA images rendered from objaverse. We follow the original VAE hyperparameters with a base learning rate of 4.5e-6 and a batch size of 64. We train the M-VAE for 60000 iterations to converge.

\mypara{Global self-attention}
Concretely, for a batch of $B$ samples with each having $N$ conditional images and $M$ generation images, the tensor size for the two branches would be $[B,N,C,H,W]$ and $[B,M,C,H,W]$, respectively, where $C, H, W$ are the number of channels, height, and width of the UNet features at a specific self-attention layer. We concatenate and reshape these tensors into a new tensor of size $[B,(N+M)*H*W,C]$, then apply global self-attention at the second dimension.
